# Supplementary material for: Fault-Tolerant Neural Networks from Biological Error Correction Codes
Source: arXiv:2202.12887 source file (2024-02-09)
Supplement: Supplementary file 1 [file supplementary.pdf]

# Supplementary information for “Biological error correction codes generate fault-tolerant neural networks”

## CONTENTS

|                                                                                |    |
|--------------------------------------------------------------------------------|----|
| I. Digital fault tolerance via concatenated repetition code                    | 1  |
| II. Fault tolerance against synaptic failure via concatenated repetition code  | 1  |
| III. Comparison of repetition for discrete versus analog fault-tolerance       | 3  |
| IV. Summary of grid codes                                                      | 3  |
| V. Fault-tolerant Gaussian-weighted neural network                             | 4  |
| VI. Demonstration of Boolean gates with modified activation functions          | 6  |
| VII. Demonstration of logical NAND threshold using ReLU activation function    | 7  |
| VIII. Concatenation with repetition code for repeated lattices                 | 8  |
| IX. Comparison of discrete and analog thresholds for formula-based computation | 9  |
| References                                                                     | 10 |

## I. DIGITAL FAULT TOLERANCE VIA CONCATENATED REPETITION CODE

We begin by presenting an adaptation of the original construction of a fault-tolerant Boolean gate via a recursive concatenation of repetition codes, initially proposed in [1] and more rigorously discussed in [2]. To best explain this scheme, let us consider a Boolean gate  $B(x)$ , where  $x$  may denote multiple bits (for instance  $\text{NAND}(x_0, x_1)$ ), and its faulty counterpart  $B_p$  that fails (i.e. outputs the incorrect bit) with probability  $p$ . We would like to construct a fault-tolerant version of  $B_p$  whose error can be decreased arbitrarily for  $p < p_0$ . This is achieved by devising a recursive concatenation scheme wherein a *logical*  $B$  gate is constructed from *physical*  $B$  gates, these being the faulty  $B_p$  gates. In particular, a logical  $B$  gate at concatenation level- $\ell$ , which we denote by  $B_p^{(\ell)}$ , is recursively defined by a mapping of gates at concatenation level  $\ell - 1$ , with the base case  $B_p^{(0)}(x) = B_p$ . In this mapping,  $B_p^{(\ell)}$  is defined as a repetition code acting on multiple outputs of  $B_p^{(\ell-1)}$ , such that the error suffered by  $B_p^{(\ell)}$  is less than that of  $B_p^{(\ell-1)}$  for  $p < p_0$ .

In his seminal work on fault tolerance, von Neumann employed a ternary repetition code, in which a logical bit is encoded as a bundle of physical bits. At concatenation level  $\ell$ , each bundle consists of  $3^\ell$  physical bits, and its corresponding logical bit may be decoded as the majority of its physical bits; for instance, 110 encodes the logical bit 1 at concatenation level  $\ell = 1$ . In this manner, the inputs and outputs to  $B_p^{(\ell)}(x)$  are bundles of size  $3^\ell$ , and the output is correct if its physical bits decode to the correct logical bit.

The recursive mapping from  $B_p^{(\ell)}$  to  $B_p^{(\ell+1)}$  is defined by this ternary repetition code: the inputs to  $B_p^{(\ell+1)}$ , which are bundles of size  $3^{\ell+1}$ , are linearly partitioned into three bundles of size  $3^\ell$ , which are then sent through  $B_p^{(\ell)}$  gates in parallel to generate nine independent output bundles (each also of size  $3^\ell$ ). To correct possible errors in the output bundles, these bundles are then split into three groups of threes, each of which is passed through a (faulty) majority voting gate, and the resulting outputs are recombined into a bundle of size  $3^{\ell+1}$  which represents the final output of  $B_p^{(\ell+1)}$ . The majority voting gate is constructed from  $B_p^{(\ell)}$  gates, and hence is also imperfect; its explicit construction depends on the Boolean gate of interest and influences the fault tolerance threshold. In general, the fewer  $B_p^{(\ell)}$ 's in the majority gate, the larger the threshold.

For clarity, we depict the application of this fault tolerance protocol to a NAND gate in Fig. S1. The specific arrangement of the wires fed into the majority voting gates is chosen to prevent error propagation and produce a nonzero threshold. Not all arrangements will yield a nonzero threshold in the limit  $\ell \rightarrow \infty$ ; von Neumann's original presentation even suggests randomly permuting these wires. As the NAND gate is universal for Boolean computation, this construction enables arbitrarily accurate computation of any Boolean function from faulty NAND gates if the failure probability  $p$  lies below the threshold  $p_0$ .

## II. FAULT TOLERANCE AGAINST SYNAPTIC FAILURE VIA CONCATENATED REPETITION CODE

In this section, we describe the details of how the aforementioned concatenated repetition code may be adapted to devise a fault-tolerant neural network robust against synaptic failure. We consider a neural network constructed from rectified linear unit (ReLU) activation functions, where  $\text{ReLU}(x) = \max(0, x)$  on real inputs  $x$ . In this case, synaptic failure may be modelled by replacing each ReLU with a faulty ReLU that fails with

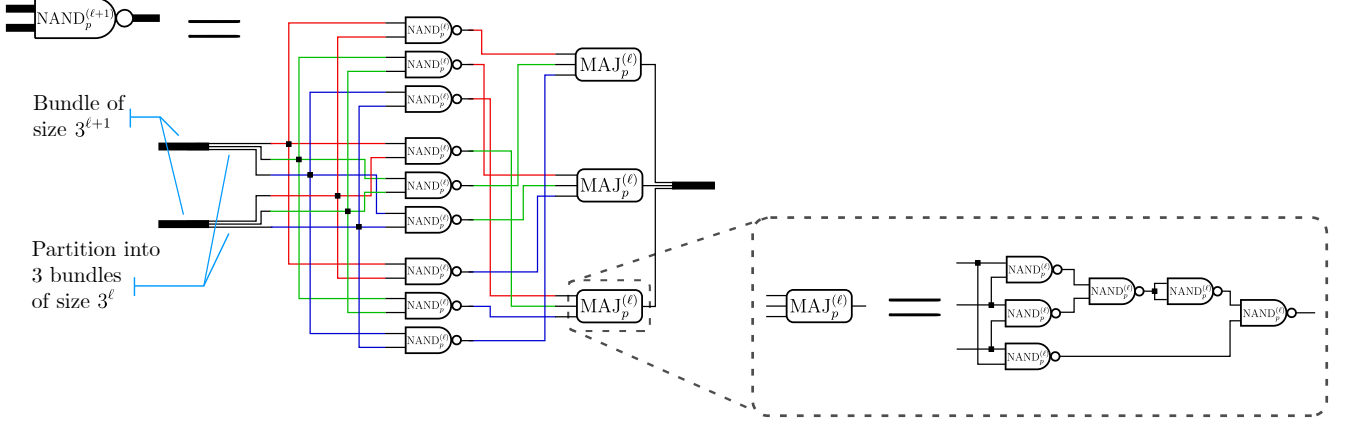

FIG. S1. The recursive concatenation scheme, based on a repetition code, used to construct a NAND at concatenation level  $\ell + 1$  (denoted  $\text{NAND}_p^{(\ell+1)}$ ) from NAND's at level  $\ell$ , with the base case  $\text{NAND}_p^{(0)} = \text{NAND}_p$ . The gates denoted  $\text{MAJ}_p^{(\ell)}$  indicate a majority voting operation, whose construction is illustrated in the inset. Note how the fault-tolerant ReLU of Fig. 2 of the main text is a generalization of this construction.

probability  $p$ , i.e.,

$$\text{ReLU}_p(x) = \begin{cases} \text{ReLU}(x) & \text{with probability } 1 - p \\ 0 & \text{with probability } p. \end{cases} \quad (\text{S1})$$

Like von Neumann's error model for Boolean gates, the output of this faulty ReLU is reliably incorrect with some probability, and thus its errors may be corrected by employing a concatenated repetition code.

The aim is to construct a fault-tolerant ReLU activation function, or equivalently a fault-tolerant neuron. We will employ a concatenated ternary repetition code analogous to that presented above, replacing each logical Boolean gate at level  $\ell$  with a logical ReLU at level  $\ell$ , which we denote by  $\text{ReLU}_p^{(\ell)}$ . However, there is one important distinction in our construction: as inputs and outputs are now analog instead of binary, we will interpret the logical value carried by a bundle as the *median* of its values. Accordingly, the majority voting gate in the original repetition code is replaced by a median gate, which will appropriately correct single errors. The complete recursive scheme is depicted in the main text in Fig. 1.

What remains is to construct the median operation out of ReLU's. At concatenation level  $\ell$ , we are interested in computing the median of three bundles, each of size  $3^\ell$ . Denoting this quantity as  $m = \text{Med}_p^{(\ell)}(a, b, c)$ , it may be computed with the following network of depth three:

$$\begin{aligned} x &= \text{ReLU}_p^{(\ell)}(a - b) \\ y &= \text{ReLU}_p^{(\ell)}(-a + c + x) \\ z &= \text{ReLU}_p^{(\ell)}(b - c + x) \\ m &= \text{ReLU}_p^{(\ell)}(a + b - c + y - z). \end{aligned} \quad (\text{S2})$$

While the final ReLU is not strictly necessary for the

computation of the median, it is included to prevent error propagation from the inputs and achieve fault tolerance. As a result, this median works only on positive inputs, but this is admissible as the output of  $\text{ReLU}_p^{(\ell)}$  (which is input into the median) is necessarily non-negative. We also note that this median construction employs skip connections to perform its computation.

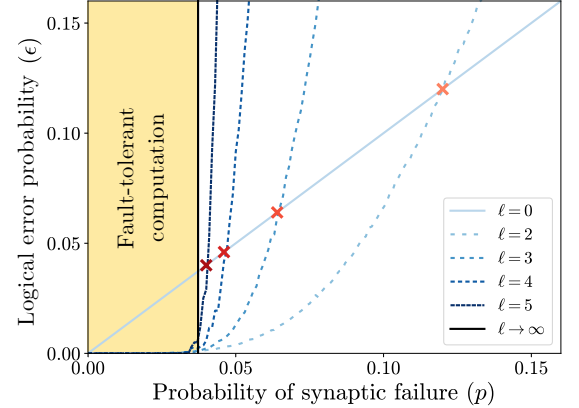

FIG. S2. The logical error probability of  $\text{ReLU}_p^{(\ell)}(x)$  on random inputs  $x \in [-1, 1]$  as determined by numerical simulation. The pseudothresholds (red crosses) occur when the error probability intersects that of  $\ell = 0$ ; they converge exponentially to the threshold  $p_0 \approx 3.72\%$  (vertical black line) with increasing  $\ell$ .

This construction ultimately produces a fault-tolerant ReLU neuron with threshold  $p_0 \approx 3.72\%$ . We visualize this threshold via the pseudothresholds generated by increasing levels of concatenation (Fig. S2). The straightforward assembly of individual fault-tolerant neurons provides a fault-tolerant neural network protected against synaptic failures.

### III. COMPARISON OF REPETITION FOR DISCRETE VERSUS ANALOG FAULT-TOLERANCE

While the repetition code is sufficient to arrive at digital fault-tolerance when subject to bit-flip errors or synaptic failure, it is insufficient for analog computation in the presence of additive Gaussian noise. Key to this is the  $\mathcal{O}(\text{polylog}(1/\epsilon))$  scaling with respect to the desired output error rate  $\epsilon$  in the definition of fault-tolerance.

For Boolean (more generally discrete) random variables, suffering from i.i.d. bit-flip errors at a rate  $p < 1/2$ , a repetition code of size  $M$  reduces errors exponentially as  $\sim p^M$ . Given a target error rate  $\epsilon$ , it is sufficient to choose

$$M \sim \frac{\log \frac{1}{\epsilon}}{\log \frac{1}{p}}. \quad (\text{S3})$$

Using the concatenation scheme described in Section I and the union bound to reduce errors to  $N/\epsilon$ , we find that this translates to the desired  $\mathcal{O}(N \log^b(N/\epsilon))$  scaling in the definition of fault-tolerance so long as the error rate is below a threshold  $p_0$  that is dependent on the details of the error correcting circuit.

For analog variables, the repetition code does not suppress errors strongly enough to achieve this scaling. For additive Gaussian noise with standard deviation  $\sigma$ , a repetition code of size  $M$  suppresses errors not exponentially in  $M$ , but only as  $\sim \sigma/\sqrt{M}$ . For a target standard deviation  $\epsilon$ , the code size is required to scale as

$$M \sim \left(\frac{\sigma}{\epsilon}\right)^2. \quad (\text{S4})$$

Analog computation using the repetition code would require an asymptotic lower bound of  $\Omega(\text{poly}(1/\epsilon))$  resources, and thus does not meet our definition of fault-tolerance. In order to achieve analog fault-tolerance, we must make use of a stronger error correcting code.

### IV. SUMMARY OF GRID CODES

For reference, we will now provide a self-contained exposition of the original grid code results [3–5]. The codespace is defined by a set of  $M$  relatively prime integers (“moduli”) denoted  $\{\lambda_j\}_{j=1}^M$ .

In a noiseless setting, the grid code encoder maps an element  $x_{i_0}$  from a set of discrete values  $\{x_i\}$  over a fixed domain  $0 \leq x_i < X$  to a codeword of phases  $\phi := \text{Enc}[x_{i_0}]$  for encoder

$$\text{Enc}[x_{i_0}] := \left\{ \phi_j = \frac{e(x_{i_0})}{\lambda_j} \bmod 1 \right\}, \quad (\text{S5})$$

where the function  $e(x_{i_0}) \in [0, X)$  is chosen to be the identity to simply represent  $x_{i_0}$ ; we will later choose non-identity  $e$  to perform computation. The choice of rela-

tively prime moduli ensures, by consequence of the Chinese Remainder Theorem, that all  $x \in [0, \prod_{j=1}^M \lambda_j)$  are encoded into distinct codewords. Restricting our domain as above, with  $X \ll \prod_{j=1}^M \lambda_j$ , allows the remaining phase space to be used for error correction. To maintain the favorable error-correcting properties of the grid code, the  $x_i$ ’s are chosen to satisfy  $x_i \ll X$ , and the minimum spacing between codewords  $\Delta x := \min_{i \neq j} |x_i - x_j|$  is chosen such that  $\max_j \lambda_j \ll \Delta x$ . More generally, when  $e(x_{i_0})$  is not the identity function, the same condition must be upheld for  $\Delta x$  given by  $\min_{i \neq j} |e(x_i) - e(x_j)|$  such that  $e(x_i) \neq e(x_j)$ . In this limit, two codewords encoding randomly sampled  $x_1, x_2 \in [0, X)$  (or  $e(x_1)$  and  $e(x_2)$ ) are well-approximated by i.i.d. samples of a uniform distribution [5]. We visualize this fact in Fig. S3.

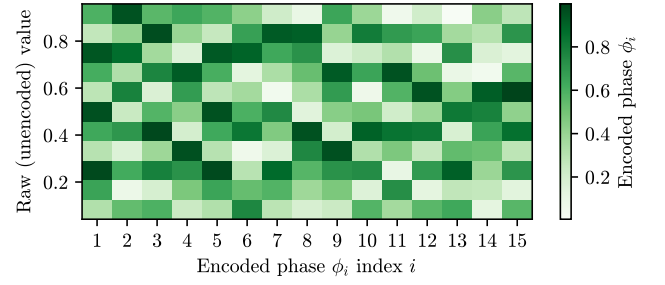

FIG. S3. Example encoding performed by the grid code over  $M = 15$  moduli  $\{\lambda_1, \dots, \lambda_{15}\}$ .

In the presence of Gaussian neural spiking noise, the noiseless encoder  $\text{Enc}[x_{i_0}]$  is replaced by the noisy encoder

$$\widetilde{\text{Enc}}[x_{i_0}] = \left\{ \tilde{\phi}_j = \frac{e(x_{i_0})}{\lambda_j} + \xi \bmod 1 \right\}, \quad (\text{S6})$$

for i.i.d.  $\xi \sim \mathcal{N}(0, \sigma)$  sampled for each phase.

We now show that the described decoding procedure, illustrated in Fig. 2b of the main text, is indeed performing maximum likelihood estimation. If  $x$  is known to belong to a discrete set of values  $\{x_i\}$ , the estimated decoding  $\hat{x}$  is given by maximizing the conditional probability

$$\hat{x} = \arg \max_{x_k} P(\phi | x_k). \quad (\text{S7})$$

The likelihood function is a wrapped normal distribution

$$P(\phi | x_k) \propto \prod_{j=1}^M \exp \left( -\frac{1}{2\sigma^2} \|\text{Enc}[x_k]_j - \phi_j\|^2 \right), \quad (\text{S8})$$

where  $\|x\| \equiv \min\{|x|, 1 - |x|\}$  denotes the distance between phases. The likelihood function is well approximated by the more tractable circular normal function in

the limit of  $\sigma \ll 1$  by

$$P(\phi|x_k) \propto \prod_{j=1}^M \exp\left(\frac{1}{2\pi\sigma^2} \cos\left[2\pi\left(\frac{x_k}{\lambda_j} - \phi_j\right)\right]\right). \quad (\text{S9})$$

Comparing Eq. S9 and Eq. 2 in the main text, we see that the neural network is maximizing the likelihood.

We summarize an analysis of the grid code's distance. Since the  $M$  phases  $\phi_j$  fall between 0 and 1, the coding space is the unit hypercube  $[0, 1]^M$ ; due to unit modulo, the coding space satisfies periodic boundary conditions and thus corresponds to the  $M$ -torus. The coding line  $[0, X)$  is thus a set of parallel line segments in the hypercube. In general, error correction codes may be described as a hypersphere packing problem: each codeword corresponds to an origin of a sphere in a high-dimensional space, and errors that fall within the radius of the sphere are correctable to the true codeword. Here, the grid code is a hypersphere packing problem in the  $M - 1$  dimensional hyperplane perpendicular to the coding line segments. Under this formalism, we arrive at a scaling of the minimum distance between line segments with the number of phases for fixed  $X$  of  $d_{\min} = \Theta(\sqrt{M})$  [5], denoting an asymptotic bound on  $d_{\min}$  from both above and below. Our choice of  $\lambda \ll \Delta x$  ensures that each  $\text{Enc}[x_i]$  lies within a different line segment and therefore is also separated by at least  $d_{\min}$ , and consequently any perturbation in the phase space less than  $d_{\min}/2$  is correctable using the maximum likelihood decoder.

## V. FAULT-TOLERANT GAUSSIAN-WEIGHTED NEURAL NETWORK

We now provide details of the computation showing the number of physical neurons required to suppress arbitrary Gaussian noise. We assume an error model where  $\xi \sim \mathcal{N}(0, \sigma)$  is added to the output of each neuron, representing the noise associated with neural spikes in a biological setting. We will be encoding an  $x_{k_0}$  that is guaranteed to belong to a discrete set of  $S$  values  $\{x_k = k\Delta x\}$  for  $k = 0, \dots, S - 1$ , such that  $(S - 1)\Delta x < X$  for some  $X$ . The moduli must satisfy  $\lambda_j \ll X \ll \prod_{j=1}^M \lambda_j$  for relatively prime  $\lambda_j$ , and thus  $x_k/\lambda_j \sim \mathcal{U}(0, 1)$  for random  $x_k$ . Additionally, we take both the number of moduli  $M$  and the number of neurons  $m_0$  connected from the previous layer to be much larger than one, allowing application of the central limit theorem.

Taking advantage of the periodicity of the grid code due to the periodicity of the phases, we introduce a smaller range of values  $[0, X')$  compared to the full range of the standard grid code  $[0, X)$ . To remain consistent with the assumptions stated above, we require  $\lambda_j \ll X' \ll \prod_{j=1}^M \lambda_j$ . Moreover, in order to maintain properties of modular arithmetic, we restrict the logical weights to integer weights  $a_i \in \mathbb{Z}$  such that  $\sum_i |a_i| \leq X/X'$ . A ReLU activation function may be implemented by the

logical activation function

$$e(x_i) = \begin{cases} 0 & (x_i \bmod X') < X'/2 \\ (x_i - X'/2) \bmod X' & (x_i \bmod X') \geq X'/2, \end{cases} \quad (\text{S10})$$

as shown in Fig. S4. This corresponds to choosing weights on the physical neurons  $W_{ij}^{\text{enc}} = \frac{e(x_i)}{\lambda_j} \bmod 1$  (red connections in Fig. 3a of the main text). However, we assume that the logical weights  $a_i$  are approximately normally distributed from a Gaussian distribution with standard deviation  $\alpha$ . (In Sec. VI, logical weights will be set to unity to implement Boolean gates.)

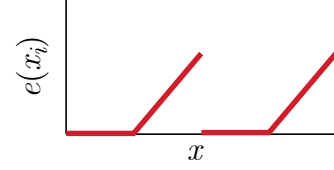

FIG. S4. Rectified linear unit (ReLU) activation function for  $X' = X/2$ . The logical ReLU activation function  $e(x_i)$  used in the encoder (Eq. S10) allows the fault-tolerant neural network to implement the standard ReLU activation function.

The general construction of the logical neuron (Fig. 3a of the main text) is as follows. A previous layer of logical neurons passes to the logical neuron a set of encoded phase vectors, where the  $i$ th input neuron is denoted  $\theta^{(i)}$ . Each input neuron  $\theta^{(i)}$  encodes a quantity that lies in  $[0, X')$  in the decoded space. A series of logical weights are applied, mapping directly from grid code phases to grid code phases. Due to the unit modulo of the grid code, this will ultimately cause a sawtooth-like activation function in the decoded space. Explicitly, this unit modulo is realized by sine and cosine activation functions in the next stage of the logical neuron: the decoder. The decoder has two roles in the logical neuron. Firstly, it performs error correction, following the grid code formalism described above. Secondly, it performs computation, introducing a nonlinearity via sine and cosine functions that impose the periodicity of the phase encoding. Moreover, the decoder does not return to the original  $[0, X')$  space; instead, it outputs a value in the larger space  $[0, X)$ , allowing the application of logical weights to decode to valid values. In the final stage of the logical neuron, we apply an encoder that returns to  $[0, X')$  by choosing appropriate weights that implement a logical activation function. Consequently, much like the decoder, the encoder both plays a role similar to the original grid code (i.e., taking  $x_i$  to a vector of phases) and is directly involved in the computational aspect of the logical neuron.

Throughout the logical neuron, synaptic failures may occur, increasing the logical error probability of the final output. Although the grid code can correct all analog errors of the form of Gaussian additive noise applied to the neural spiking output, these synaptic failures cannot

be reliably corrected. In the standard neural network described in this section, we do not address the synaptic failures. However, in the neural implementation of the NAND gate (Sec. VII), we apply the standard fault-tolerant NAND construction of Evans and Pippenger [6] to correct for synaptic failures. This also provides a reconciliation with von Neumann’s traditional approach to fault tolerance, where all computations occur within the codespace: a fully fault-tolerant neural network is achieved by combining the traditional concatenated repetition code and the grid code, ensuring that the computation does indeed remain in a protected codespace throughout the entire computation.

The above framework is now made explicit to demonstrate the fault-tolerant properties of the logical neuron. Working in the codespace, the  $m_0$  neurons from the previous layer connected to the logical neuron are represented by codewords  $\text{Enc}[x_1], \dots, \text{Enc}[x_{m_0}]$ . Letting  $\text{Enc}[x_i] = \{\theta_j^{(i)}\}$  for  $j = 1, \dots, M$ , we must map from the  $m_0 \times M$  neurons in  $\{\text{Enc}[x_i]\}$  to a single set of phases  $\{\phi_j\}$  such that our activation function is applied *after* decoding and re-encoding (since the encoder applies the ReLU activation function). By assigning weights  $W_{ij} = a_i$  from  $\theta_j^{(i)}$  to  $\phi_j$  with a linear activation function and bias  $-\frac{X'}{\lambda_j} \sum_{i:a_i < 0} a_i$ , we obtain phases in the absence of noise:

$$\phi_j = \left( \sum_i a_i \theta_j^{(i)} \right) - \left( \frac{X'}{\lambda_j} \sum_{i:a_i < 0} a_i \right). \quad (\text{S11})$$

Adding in noise, we denote a noisy encoding by phases  $\tilde{\theta}_j^{(i)}$ . Each of the  $S$  neurons over the discretized decoded space have noise  $\xi$ , and each is multiplied by approximately uniformly distributed weights due to the phases over the moduli. Applying the central limit theorem to  $\sum_{i=1}^S u\xi$  for  $u \sim \mathcal{U}(0, 1)$ , we find mean zero noise with variance  $\sigma^2 \cdot S/3$ . (For simplicity of notation, we drop the subscript on each  $\xi$  denoting the i.i.d. random variables.) Adding the noise of the codespace neuron to the noise acquired from the plaintext neuron, we find  $\tilde{\theta}_j^{(i)} = \theta_j^{(i)} + \xi + \zeta$  for  $\zeta \sim \mathcal{N}(0, \sigma\sqrt{S/3})$ . Inserting noise in Eq. S11, we have

$$\begin{aligned} \tilde{\phi}_j &= \left[ \sum_{i=1}^{m_0} a_i \tilde{\theta}_j^{(i)} \right] - \left( \frac{X'}{\lambda_j} \sum_{i:a_i < 0} a_i \right) + \xi \\ &= \phi_j + \xi + \sum_{i=1}^{m_0} a_i (\xi + \zeta). \end{aligned} \quad (\text{S12})$$

Applying the central limit theorem to the noise interacting with the neural network weights  $a_i$ , we find that the mean vanishes and  $\text{Var}[\sum_{i=1}^{m_0} a_i (\xi + \zeta)] = \frac{1}{3} S m_0 \alpha^2 \sigma^2$ . To simplify notation, we introduce the variable  $a = 4\pi^2(1 + S m_0 \alpha^2/3)$ .

The error correction  $\tilde{\phi}' = \widetilde{\text{Enc}}[\widetilde{\text{Dec}}[\tilde{\phi}]]$  will produce the correct codeword with error  $\xi$  on each phase — as

was assumed in the logical neuron input — if  $\text{Dec}[\tilde{\phi}]$  identifies the correct value. The decoder shown in Fig. 3a of the main text uses two layers, which we now make explicit. The first layer multiplies each  $\phi_j$  with weight  $2\pi$ ; the second layer uses periodic activation functions to compute  $\sin(2\pi\phi_j)$  and  $\cos(2\pi\phi_j)$  respectively multiplied with weights  $W_{jk}^{\sin} = \sin\left(2\pi\frac{x_k}{\lambda_j}\right)$  and similarly  $W_{jk}^{\cos} = \cos\left(2\pi\frac{x_k}{\lambda_j}\right)$ . After applying the final step activation function to obtain a decoding, the error is ‘reset’ if the decoding  $\widetilde{\text{Dec}}[\tilde{\phi}]$  is successful: the logical neuron will not propagate any additional noise into future computations. Evaluating all noise contributions, we have

$$\text{Dec}[\tilde{\phi}] = \arg \max_k f(k), \quad (\text{S13})$$

$$f(k) := \xi + \sum_{j=1}^M [f_1(j, k) + f_2(j, k)], \quad (\text{S14})$$

where

$$f_1(j, k) = \sin\left(2\pi\frac{x_k}{\lambda_j}\right) \left[ \sin\left(2\pi\tilde{\phi}_j\right) + \xi \right], \quad (\text{S15})$$

$$f_2(j, k) = \cos\left(2\pi\frac{x_k}{\lambda_j}\right) \left[ \cos\left(2\pi\tilde{\phi}_j\right) + \xi \right], \quad (\text{S16})$$

and as usual each  $\xi$  is sampled i.i.d.

Suppose that the correct neuron value corresponds to  $k = k_0$ . For the decoder to identify the correct neuron via a threshold cutoff, we require  $f(k_0) > f(k \neq k_0)$  for all  $k$ . If the mean of the correct neuron is greater than the mean of each incorrect neuron, a threshold will exist to distinguish the correct decoding from incorrect decodings in expectation. We use this to gain an analytical scaling for  $M(\epsilon)$  here; a more detailed treatment of the threshold is found in the analysis of the logical NAND.

The key observation is that the noiseless phases  $\phi_j$  are given by  $\phi_j = x_{k_0}/\lambda_j \bmod 1$ . At  $k = k_0$ , this phase aligns with the neural network weights  $\sin\left(2\pi\frac{x_{k_0}}{\lambda_j}\right)$  or  $\cos\left(2\pi\frac{x_{k_0}}{\lambda_j}\right)$ . On the other hand, at all  $k \neq k_0$ , the neural network weights are sine or cosine of a uniformly distributed random variable.

Formalizing this argument, we find that the true decoding is centered away from zero:

$$\begin{aligned} f(k_0) &\sim \mathcal{N}\left(Me^{-a\sigma^2/2}, \right. \\ &\quad \left. \sqrt{M\left(\frac{1}{2} + \frac{1}{2}e^{-2a\sigma^2} - e^{-a\sigma^2} + \sigma^2\right) + \sigma^2}\right), \end{aligned} \quad (\text{S17})$$

while the incorrect decoding is centered at zero:

$$f(k \neq k_0) \sim \mathcal{N}\left(0, \sqrt{M\left(\frac{1}{2} + \sigma^2\right) + \sigma^2}\right), \quad (\text{S18})$$

where both distributions are seen to have standard deviations  $\mathcal{O}(\sqrt{M})$ . Upper-bounding the maximum element drawn from the distribution of  $f(k \neq k_0)$  out of  $S$  draws using Jensen's inequality and a union bound, we find that

$$f_{\max}(k \neq k_0) := \mathbb{E}[\max \text{ draw of } f(k \neq k_0)] \quad (\text{S19})$$

$$\leq \sqrt{[M(1 + 2\sigma^2) + 2\sigma^2] \log S}. \quad (\text{S20})$$

Finally, to determine if  $\arg \max_k$  returns a value other than  $k_0$ , we compute the probability that this exceeds  $f(k_0)$ :

$$\begin{aligned} \Pr[\text{logical neuron fails}] &= \Pr[f(k_0) < f_{\max}(k \neq k_0)] \\ &\leq \frac{1}{2} \operatorname{erfc} \frac{e^{-a\sigma^2/2} M - \sqrt{[M(1 + 2\sigma^2) + 2\sigma^2] \log S}}{\sqrt{M(1 + e^{-2a\sigma^2} - 2e^{-a\sigma^2} + 2\sigma^2) + 2\sigma^2}}. \end{aligned} \quad (\text{S21})$$

Expanding in small  $\epsilon$  and taking  $M, a\sigma^2 \gg 1$ , we find that

$$\begin{aligned} M(\epsilon) &\approx \log(1/\epsilon) \left[ e^{a\sigma^2} (1 + 2\sigma^2) + e^{-a\sigma^2} - 2 \right] \\ &\approx e^{a\sigma^2} (1 + 2\sigma^2) \log(1/\epsilon), \end{aligned} \quad (\text{S22})$$

consistent with Eq. 3 of the main text. The number of neurons is linear in the number of moduli due to the structure of the logical neuron (see Fig. 3a of the main text).

## VI. DEMONSTRATION OF BOOLEAN GATES WITH MODIFIED ACTIVATION FUNCTIONS

While the neural network presented above is a universal approximator of continuous functions due to the use of a ReLU activation function, we demonstrate the flexibility of the fault-tolerant network construction and implement different activation functions amenable to the neural evaluation of Boolean gates. (The ReLU neural network is also used to implement a NAND gate in the following section.) By constructing a universal set of Boolean gates with fault-tolerant neural networks, any Boolean circuit can be implemented up to arbitrarily small error in the presence of arbitrarily large noise.

A natural construction for Boolean gates emerges if additional encoders that implement different activation functions are introduced. We will show how to generate the activation functions in Fig. 3b of the main text, which will ultimately allow the neural implementation of a multiplier circuit (Fig. S5 and Fig. 3c).

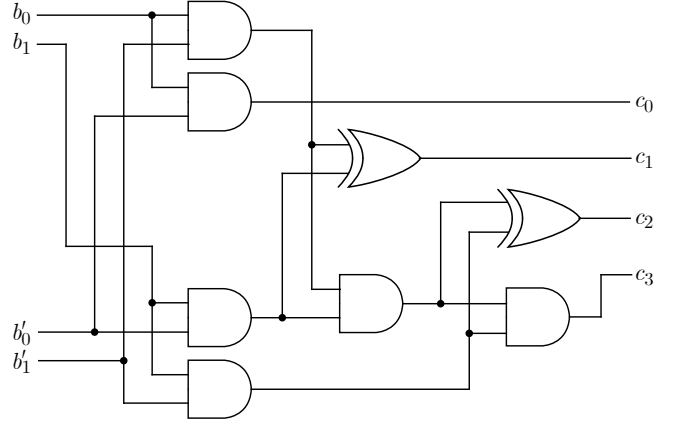

FIG. S5. Two-bit multiplication circuit decomposed into six AND gates and two XOR gates. As shown in Fig. 4 of the main text, a fault-tolerant neural network assembled of neural Boolean gates satisfies the fault-tolerant neural network theorem with  $\mathcal{O}(e^{\mathcal{O}(\sigma^2)})$  physical neurons. Two 2-bit binary numbers  $b_0b_1$  and  $b'_0b'_1$  are provided as input to the circuit, and the output product  $c_0c_1c_2c_3$  is returned. Here, the 0 index denotes the least significant bit.

Define two logical input bits  $A, B \in \{0, a\}$ , interpreting 0 as False and  $a$  as True. Letting  $\Delta x = a$ , the decoder  $\text{Dec}[\phi]$  will only decode to the set of variables  $\{x_1 = 0, x_2 = a, x_3 = 2a\}$ . For notational convenience, we define codeword vectors

$$\phi_a := \left\{ \phi_j = \frac{a}{\lambda_j} \bmod 1 \right\}, \quad (\text{S23})$$

$$\phi_0 := \left\{ \phi_j = \frac{0}{\lambda_j} \bmod 1 \right\}. \quad (\text{S24})$$

Beginning with a NOT gate, define the NOT encoder  $\text{Enc}^\neg[x_1] = \phi_a$  and  $\text{Enc}^\neg[x_2] = \text{Enc}^\neg[x_3] = \phi_0$ . As before, this corresponds to a neural network with weights given by the codeword vectors. To compute  $\neg A$ , we simply compute  $\text{Enc}^\neg[\text{Dec}[A]]$  to apply the error correction and re-encode into the codespace with a NOT computation.

To implement AND and OR gates, we require an additional layer of unity weights, giving  $\phi_i = \theta_i^A + \theta_i^B$ . Applying the decoder will give either 0,  $a$  or  $2a$  based on the cases  $(A, B) \in \{(0, 0)\}, \{(a, 0), (0, a)\}$  or  $\{(a, a)\}$  respectively. The AND encoder is given by  $\text{Enc}^\wedge[x_1] = \text{Enc}^\wedge[x_2] = \phi_0$  and  $\text{Enc}^\wedge[x_3] = \phi_a$ , and the OR encoder is given by  $\text{Enc}^\vee[x_1] = \phi_0$  and  $\text{Enc}^\vee[x_2] = \text{Enc}^\vee[x_3] = \phi_a$ .

Although AND, OR, and NOT form a universal gate set, we also include XOR for direct use in the two-bit multiplier, given by  $\text{Enc}^\oplus[x_1] = \text{Enc}^\oplus[x_3] = \phi_0$  and  $\text{Enc}^\oplus[x_2] = \phi_a$ . Using these neural gates, we implement the two-bit multiplier shown in Fig. S5.

## VII. DEMONSTRATION OF LOGICAL NAND THRESHOLD USING RELU ACTIVATION FUNCTION

Above, we used natural constructions of Boolean gates through a careful choice of activation function in the codespace. For completeness, we demonstrate here the universality of the fault-tolerant neural network with a ReLU activation function and construct a NAND gate, which allows the implementation of arbitrary Boolean formulas. As seen in the NAND gate activation function of Fig. 3b, the NAND activation function is the opposite of the standard ReLU activation function. Hence, unlike the construction for Boolean formulas described in the previous section, we choose 0 to correspond to the True state and  $a$  to the False state. This makes the ReLU activation function equivalent to the direct implementation of a NAND gate.

Repeating the noisy logical neuron analysis but with logical weights  $a_i = 1$  and three decoder neurons, a similar analysis shows that Eq. S17 is replaced by

$$f_{\text{NAND}}(k_0) \sim \mathcal{N}\left(M \cdot \frac{e^{-6\pi^2\sigma^2} \text{erf}^6(\sqrt{2}\pi\sigma)}{512\pi^3\sigma^6}, \sqrt{M\left(\frac{1}{2} + \sigma^2 - \zeta\right) + \sigma^2}\right), \quad (\text{S25})$$

for

$$\zeta = \frac{e^{-12\pi^2\sigma^2} \text{erf}^{12}(\sqrt{2}\pi\sigma) - 4\pi^3\sigma^6 e^{-24\pi^2\sigma^2} \text{erf}^6(2\sqrt{2}\pi\sigma)}{262144\pi^6\sigma^{12}}. \quad (\text{S26})$$

However, Eq. S18 remains unchanged, i.e.

$$f_{\text{NAND}}(k \neq k_0) \sim \mathcal{N}\left(0, \sqrt{M\left(\frac{1}{2} + \sigma^2\right) + \sigma^2}\right). \quad (\text{S27})$$

Repeating the analysis above to estimate  $\text{Pr}[f_{\text{NAND}}(k_0) < f_{\text{NAND}}(k \neq k_0)]$  yields the number of moduli

$$M(\epsilon) \approx \frac{262144\pi^6 e^{12\pi^2\sigma^2} \sigma^{12} (4\sigma^2 + 1) \log\left(\frac{3}{\epsilon}\right)}{\text{erf}^{12}(\sqrt{2}\pi\sigma)} \quad (\text{S28})$$

$$= \mathcal{O}\left(e^{a\sigma^2} \log(1/\epsilon)\right), \quad (\text{S29})$$

consistent with the result for a Gaussian-weighted neural network.

To account for synaptic failure with probability  $p$ , we must modify Eqs. S25 and S27. While a functional synapse with additive Gaussian neural spiking error returns value  $y + \xi$ , a synaptic failure returns value 0. We proceed to treat each case of the effect of synaptic failure for each possible type of synapse in Fig. 3a of the main text. The goal is to find an upper bound on the probability that the logical NAND fails, corresponding to a lower bound on the threshold for synaptic failure.

Considering the synapses from the decoder neurons  $x_i$  to the new logical phases  $\phi_j'$  (i.e., the final layer of Fig. 3a), a failed synapse may originate from the correct decoder neuron or an incorrect decoder neuron. We ignore the failed synapse from an incorrect decoding, consistent with upper-bounding the failure probability. If the correct decoding fails, the encoded phase may not fire. In the application of logical weights to the logical phase of the next neuron (i.e., the first layer of Fig. 3a), the synapse with a logical weight  $a_i$  may similarly fail. The two phenomena of a correct decoder synapse failing and a logical weight synapse failing produce the same outcome: an input phase  $\theta_i^{(1,2)}$  may fail. The effect of only a single input phase (e.g.  $\theta_i^{(1)}$ ) failing is different from the effect of both input phases failing (i.e.  $\theta_i^{(1)}$  and  $\theta_i^{(2)}$ ). If one input phase fails, the logical phase  $\phi_i$  assumes a uniformly random value from 0 to 1. This has no impact on  $f_{\text{NAND}}(k \neq k_0)$ , but it reduces the mean of  $f_{\text{NAND}}(k = k_0)$  by removing a modulus and requires adjustment of the standard deviation by the inclusion of a random phase. If both input phases fail, the logical phase does not fire. Hence, a modulus is removed from both  $f_{\text{NAND}}(k \neq k_0)$  and  $f_{\text{NAND}}(k = k_0)$ . In total,  $4Mp(1-p)$  single input phases are expected to fail and  $2Mp^2$  double input phases are expected to fail.

Consider the synapses into and out of the  $\sin 2\pi\phi_i$  and  $\cos 2\pi\phi_i$ . Here, we also find two cases: if there is a failure of a single sine or cosine, the original distribution must be compensated by the remaining sine or cosine of the phase; if there is a failure of both, the modulus is removed entirely. In expectation,  $2Mp(1-p)$  failures are expected for the former effect (for each of sine and cosine), and  $2Mp^2$  failures are expected for the latter.

By adding each of the failure modes independently, we place an upper bound on logical failure due to double-counting failures that happen sequentially in the network. To evaluate the final distributions  $f'_{\text{NAND}}(k \neq k_0)$  and  $f'_{\text{NAND}}(k = k_0)$  that account for synaptic failure, we assume a large number of moduli  $M \gg 1$  and apply the central limit theorem. This produces a new set of distributions, e.g.,

$$f'_{\text{NAND}}(k \neq k_0) = \mathcal{N}\left(0, \sqrt{\sigma^2 - \frac{1}{2}M(2p(p+1) - 1)(2\sigma^2 + 1)}\right). \quad (\text{S30})$$

We now provide a more careful treatment of the activation function required for the error correction step of the logical neuron. In a biological discussion of the grid code, winner-take-all dynamics are often used to describe the decoding process [5]. However, for transparency in the treatment of noise, we demonstrate how a local step activation function can replace winner-take-all dynamics with a simpler decoder.

Since  $f'_{\text{NAND}}(k \neq k_0)$  is centered at zero with standard

deviation  $\mathcal{O}(\sqrt{M})$ , and  $f'_{\text{NAND}}(k = k_0)$  is centered at  $\mathcal{O}(M)$  with standard deviation  $\mathcal{O}(\sqrt{M})$ , we may choose a cutoff  $c$  that maximizes the probability of distinguishing between correct and incorrect decodings. Since there are three decoding neurons, a correct decoding requires the two incorrect neurons sampled from  $f'_{\text{NAND}}(k \neq k_0)$  to lie below  $c$  and the correct neuron to sampled from  $f'_{\text{NAND}}(k = k_0)$  to exceed  $c$ . Evaluating such probabilities is straightforward due to  $f'_{\text{NAND}}$  being normally distributed in both cases. This is performed analytically in Fig. 4b for the dashed line, while the cutoff is estimated numerically in the shaded region and in Fig. 4c.

Evaluated explicitly in terms of neural spiking noise standard deviation  $\sigma$  and probability of synaptic failure  $p$ , the probability that the logical NAND neuron succeeds is given by

$$\frac{1}{8} \left( \operatorname{erf} \left( \frac{c}{\sqrt{2\sigma^2 - M(2p(p+1) - 1)(2\sigma^2 + 1)}} \right) + 1 \right)^2 \times \operatorname{erfc} \left\{ \left( 512\pi^3 c \sigma^6 - e^{-6\pi^2 \sigma^2} M(2(p-3)p+1) \operatorname{erf}(\sqrt{2\pi}\sigma)^6 \right) \right. \\ \left. \left/ \left[ - \left( 2M(p(3p-7)+1) e^{-24\pi^2 \sigma^2} \left( e^{12\pi^2 \sigma^2} \times \operatorname{erf}(\sqrt{2\pi}\sigma)^{12} - 4\pi^3 \sigma^6 \operatorname{erf}(2\sqrt{2\pi}\sigma)^6 \right) \right) \right] \right. \right. \\ \left. \left. - 262144\pi^6 \sigma^{12} (M(2p(p+1) - 1)(2\sigma^2 + 1) - 2\sigma^2) \right]^{1/2} \right\}, \quad (\text{S31})$$

where the decoding step activation function cutoff  $c$  is obtained by maximizing the probability of success over all possible values of  $c$ .

To obtain the fault-tolerance threshold in Fig. 4b, we apply the result of Evans and Pippenger [6] for fault-tolerant Boolean formulas of NAND gates, which are possible if and only if the NAND probability of failure is below  $\epsilon_0 = (3 - \sqrt{7})/4$ . While the NAND construction only considers errors as bit flips — i.e., an error is triggered if a gate that should return 0 returns a 1, and vice versa — errors in the neural NAND gate are biased. (This occurs since synaptic failures bias neurons towards zero output; if all neurons fail, the neural NAND defaults to 0.) However, biased errors are strictly easier to correct than unbiased errors, and thus the threshold of Evans and Pippenger serves as an appropriate lower bound. To ensure the lower bound is applied correctly, we report the error rate of the neural NAND in a manner that counts zero output forced by synaptic failure as an error. In Fig. 4b of the main text, the quantity in Eq. S31 is compared to the threshold at  $M = 10^5$ , allowing a threshold contour to be determined in  $\sigma$  and  $p$ . This is seen to agree with the numerical simulation.

## VIII. CONCATENATION WITH REPETITION CODE FOR REPEATED LATTICES

In the previous section, we constructed a neural NAND that uses  $M$  moduli (or lattices), where each modulus is included only once. Grid cells in the mammalian cortex contain  $10^3$  to  $10^4$  repetitions of each lattice [4]. We thus examine a concatenation of the grid code with a repetition code, distinct from that of Fig. 1b in the main text (i.e., distinct from the von Neumann construction). To develop a precise construction, this requires several modifications to the above neural NAND gate. Roughly speaking, the central limit theorem reduces the variance  $\sigma^2$  to  $\sigma^2/R$ , which can drastically reduce the number of moduli required to suppress noise (Fig. 4c of the main text).

Taking the logical neuron in Fig. 3a of the main text, the main modification is to replace each phase with  $R$  copies of the phase. Each successive layer then averages over the repetitions of the previous layer, correcting for the synaptic failure probability. For example, consider  $R$  copies of the first phase  $\{\theta_{1,i}^{(1)}\}_{i=1}^R$  and  $R$  copies of the second phase  $\{\theta_{1,i}^{(2)}\}_{i=1}^R$ . In the absence of the repetition code, the phase  $\phi_1$  would be computed as  $\phi_1 = \theta_1^{(1)} + \theta_2^{(1)}$ . With the repetition code and a synaptic failure probability  $p$ , we instead choose

$$\phi_{1,j} = \frac{1}{R} \times \frac{1}{1-p} \sum_{i=1}^R \theta_{1,i}^{(1)} + \theta_{1,i}^{(2)} \quad (\text{S32})$$

and evaluate the sum for each  $\{\phi_{1,j}\}_{j=1}^R$ , ensuring that i.i.d. sampling of the Gaussian noise over  $R$  repetitions will reduce the standard deviation from  $\sigma^2$  to  $\sigma^2/R$ .

The only remaining modification is the use of step activation functions to perform a majority vote over repetitions in the final layer. As shown in Fig. 3a of the main text, the output phases are computed from the  $x_i$  returned by the decoder. For the NAND gate in the absence of repetitions, the outputs  $x_1$  (corresponding to 0),  $x_2$  (corresponding to  $a$ ), and  $x_3$  (corresponding to  $2a$ ) are multiplied by respective weights  $1/\lambda_j$ ,  $1/\lambda_j$ , and 0. We wish to prevent continuous errors in the phases further down the network. If the mean corrected by  $1/(1-p)$  were computed, the phases in the next layer may be offset by the fraction of synaptic failures differing from  $1/(1-p)$ .

To reduce errors to simple bit flips plus Gaussian noise, we replace the weight vector  $(1/\lambda_j, 1/\lambda_j, 0)/(1-p)$  with a step activation function. Since the weight associated with  $2a$  is zero, we do not connect  $x_3$  to the following layer of neurons. If  $x_1$  is selected, its mean is 0; if  $x_2$  is selected, its mean is  $a/(1-p)$ . The neurons  $\phi'_i$  receive input passed through a step function to distinguish between the two possibilities, where the location of the step is identified by an equal number of standard deviations separating the two distributions of  $x_1$  and  $x_2$ . If a sufficient number

of the  $R$  repetitions of  $x_i$  are activated, the step function will set the input value to  $\phi'_i$  to 0 or  $a$  then divide by  $\lambda_j$ . Gaussian additive noise is then applied.

As before, errors are biased due to synaptic failure setting neurons to zero; hence, the threshold of Evans and Pippenger places a lower bound on the true threshold of the neural NAND, where zero output incurred by synaptic failure is appropriately counted as a logical error. In our numerical experiments, we use  $M = 10$  moduli to remain within the biologically relevant regime. Since the central limit theorem performs poorly with a small number of moduli, an analytic approximation does not replicate numerical simulation. Nevertheless, for sufficiently large  $R = O(1000)$ , we find that the asymptotic scaling of  $\sigma^2 \rightarrow \sigma^2/R$  is satisfied (Fig. S6).

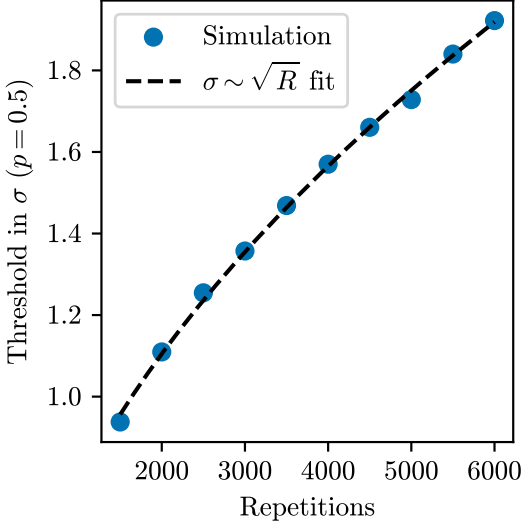

FIG. S6. Numerical simulation of the threshold as a function of the number of repetitions  $R$  per lattice. The fit shows that fault-tolerant neural network agrees with the expected scaling of  $\sigma = O(\sqrt{R})$ .

## IX. COMPARISON OF DISCRETE AND ANALOG THRESHOLDS FOR FORMULA-BASED COMPUTATION

Finally, we analyze a simple analog model of Boolean formula-based fault-tolerant computation which establishes a baseline for comparing discrete and analog thresholds. This is independent of neural computation, but rather serves as a pedagogical comparison of digital and analog computation that allows analog Gaussian noise to be translated into the well-known failure probability thresholds of Evans and Pippenger [6] using 2-input NAND gates. Accordingly, the thresholds found below do not correspond to fault-tolerant neural network thresholds.

For the following analysis, we consider a binary alphabet encoded into real-valued signals  $\{-1, 1\}$  corre-

sponding to the Boolean 0 and 1 respectively. For convenience we define the Boolean NAND to operate on our alphabet, and therefore it can be viewed as a function  $\text{NAND} : \{-1, 1\} \times \{-1, 1\} \rightarrow \{-1, 1\}$ . There is considerable freedom in defining the analog NAND gate. We will choose to analyse the noise thresholds of two representative candidates, dNAND and aNAND defined below, and argue that these are extremal in the sense that all other reasonable definitions of the analog NAND result thresholds intermediate to the ones presented.

First, consider the dNAND defined as follows:

$$\text{dNAND}_\sigma(x, y) := \text{NAND}(\text{sgn}(x), \text{sgn}(y)) + \xi, \quad (\text{S33})$$

where NAND is the noiseless Boolean NAND defined above, and sgn is the sign function. One can verify that a formula composed of dNAND gates works exactly a discrete NAND with an effective error rate  $\epsilon = \Pr[\xi \geq 1]$ . Therefore denoising is successful as long as

$$\frac{1}{2} \left[ 1 - \text{erf} \left( \frac{1}{\sigma\sqrt{2}} \right) \right] < \epsilon_0, \quad (\text{S34})$$

where  $\epsilon_0 = \frac{3-\sqrt{7}}{4}$  denotes the threshold of [6]. Numerically, we find a corresponding analog threshold of  $\sigma < \sigma_d^*$  for  $\sigma_d^* \approx 0.7409$ .

For comparison, consider the aNAND gate defined as follows:

$$\text{aNAND}_\sigma(x, y) := \frac{1 - x - y - xy}{2} + \xi \quad (\text{S35})$$

where  $\xi \sim \mathcal{N}(0, \sigma^2)$ . Note that for  $\sigma = 0$  the analog NAND gate behaves as a noiseless NAND. In this notation, the balanced depth-2 binary tree denoiser used by Evans and Pippenger [6] is written

$$\begin{aligned} \text{Denoise}_\sigma(x_1, x_2, x_3, x_4) = \\ \text{aNAND}_\sigma(\text{aNAND}_\sigma(x_1, x_2), \text{aNAND}_\sigma(x_3, x_4)). \end{aligned} \quad (\text{S36})$$

We would like to analyze the behavior of the denoiser for real-valued i.i.d. random variables  $X_i$  with  $\mathbb{E}[X_i] = x \in \{-1, 1\}$  and  $\text{Var}(X_i) = \alpha^2$ . Define  $Y := \text{Denoise}_\sigma(X_1, X_2, X_3, X_4)$ ; note that  $\mathbb{E}[Y]$  is a quartic polynomial in  $x$  plotted in Fig. S7. One finds that the denoising operation is unbiased (i.e.  $\mathbb{E}[Y] = x$ ) and has variance that depends on  $x$ : for  $x = -1$ ,

$$\text{Var}(Y) = \frac{1}{64} (\alpha^8 + 8\alpha^4 (\sigma^2 + 4) + 16\sigma^2 (\sigma^2 + 12)), \quad (\text{S37})$$

and for  $x = +1$ ,

$$\text{Var}(Y) = \frac{1}{64} (\alpha^4 + 8\alpha^2 + 4\sigma^2)^2 + \sigma^2. \quad (\text{S38})$$

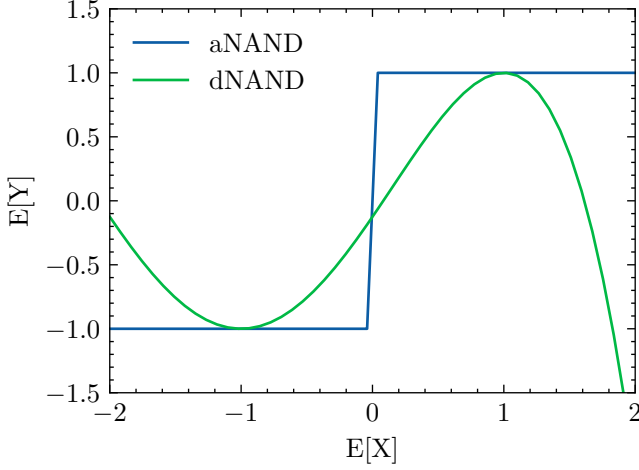

FIG. S7. A comparison of the denoiser response derived from the two proposed analog NAND gates.

Denoising is successful if  $\text{Var}(Y) < \alpha^2$  for  $x \in \{-1, 1\}$ . As in the discrete case, for  $\sigma < \sigma'_a$ , the denoiser has two fixed points, with the lower one being stable. At the denoising threshold, a saddle-node bifurcation occurs and denoising is no longer possible. Numerically, we find the denoising threshold for the aNAND to be at  $\sigma'_a \approx 0.3929$ .

For fault-tolerant computation, we require not only that denoising can be done successfully, but that at least one step of computation can be applied between denoising stages without exceeding the capacity of our denoiser. In terms of the denoising fixed points, we require that a single aNAND gate with input variances near the lower fixed point produces a resulting value that below the upper fixed point. The critical case is that where aNAND is given inputs of opposite value. Numerically we find that computation is possible below  $\sigma_a^* \approx 0.3385$ .

As in the discrete case, computation below threshold is possible with minimal overhead. Since we are assuming a formula-based model of computation, the overhead in question corresponds to an increase in depth. To arrive a rough estimate of the overhead required for denoising, note that the distance between the upper and lower fixed points for gate noise  $\sigma$  below threshold is  $\Theta(\sigma_a^{*2} - \sigma^2)$ ; additionally, each denoising step reduces the variance by a factor  $1 - \Theta(1)$ . Therefore, we find a modest depth increase by factor

$$L_a = \Theta \left( \frac{1}{\sigma_a^{*2} - \sigma^2} \log \left( \frac{1}{\sigma_a^{*2} - \sigma^2} \right) \right), \quad (\text{S39})$$

which establishes a fault-tolerance theorem for Boolean formulas composed of noisy analog NAND gates and is a similar form to the factor found by Evans and Pippenger [6] for the case of computation with discrete NAND gates.

- 
- [1] J. von Neumann, “Probabilistic logics and the synthesis of reliable organisms from unreliable components,” in *Automata Studies. (AM-34), Volume 34*, edited by C. E. Shannon and J. McCarthy (Princeton University Press, 2016) pp. 43–98.
  - [2] S. Winograd and J. D. Cowan, *Reliable computation in the presence of noise* (MIT Press Cambridge, Mass., 1963).
  - [3] T. Hafting, M. Fyhn, S. Molden, M.-B. Moser, and E. I. Moser, *Nature* **436**, 801 (2005).
  - [4] I. R. Fiete, Y. Burak, and T. Brookings, *Journal of Neuroscience* **28**, 6858 (2008).
  - [5] S. Sreenivasan and I. Fiete, *Nature Neuroscience* **14**, 1330 (2011).
  - [6] W. Evans and N. Pippenger, *IEEE Transactions on Information Theory* **44**, 1299 (1998).
